# Supplementary material for: Multimode photon blockade
Source: arXiv:2010.15292 source file (2020-10-29)
Supplement: Supplementary file 1 [file Supp_Fig1.pdf]

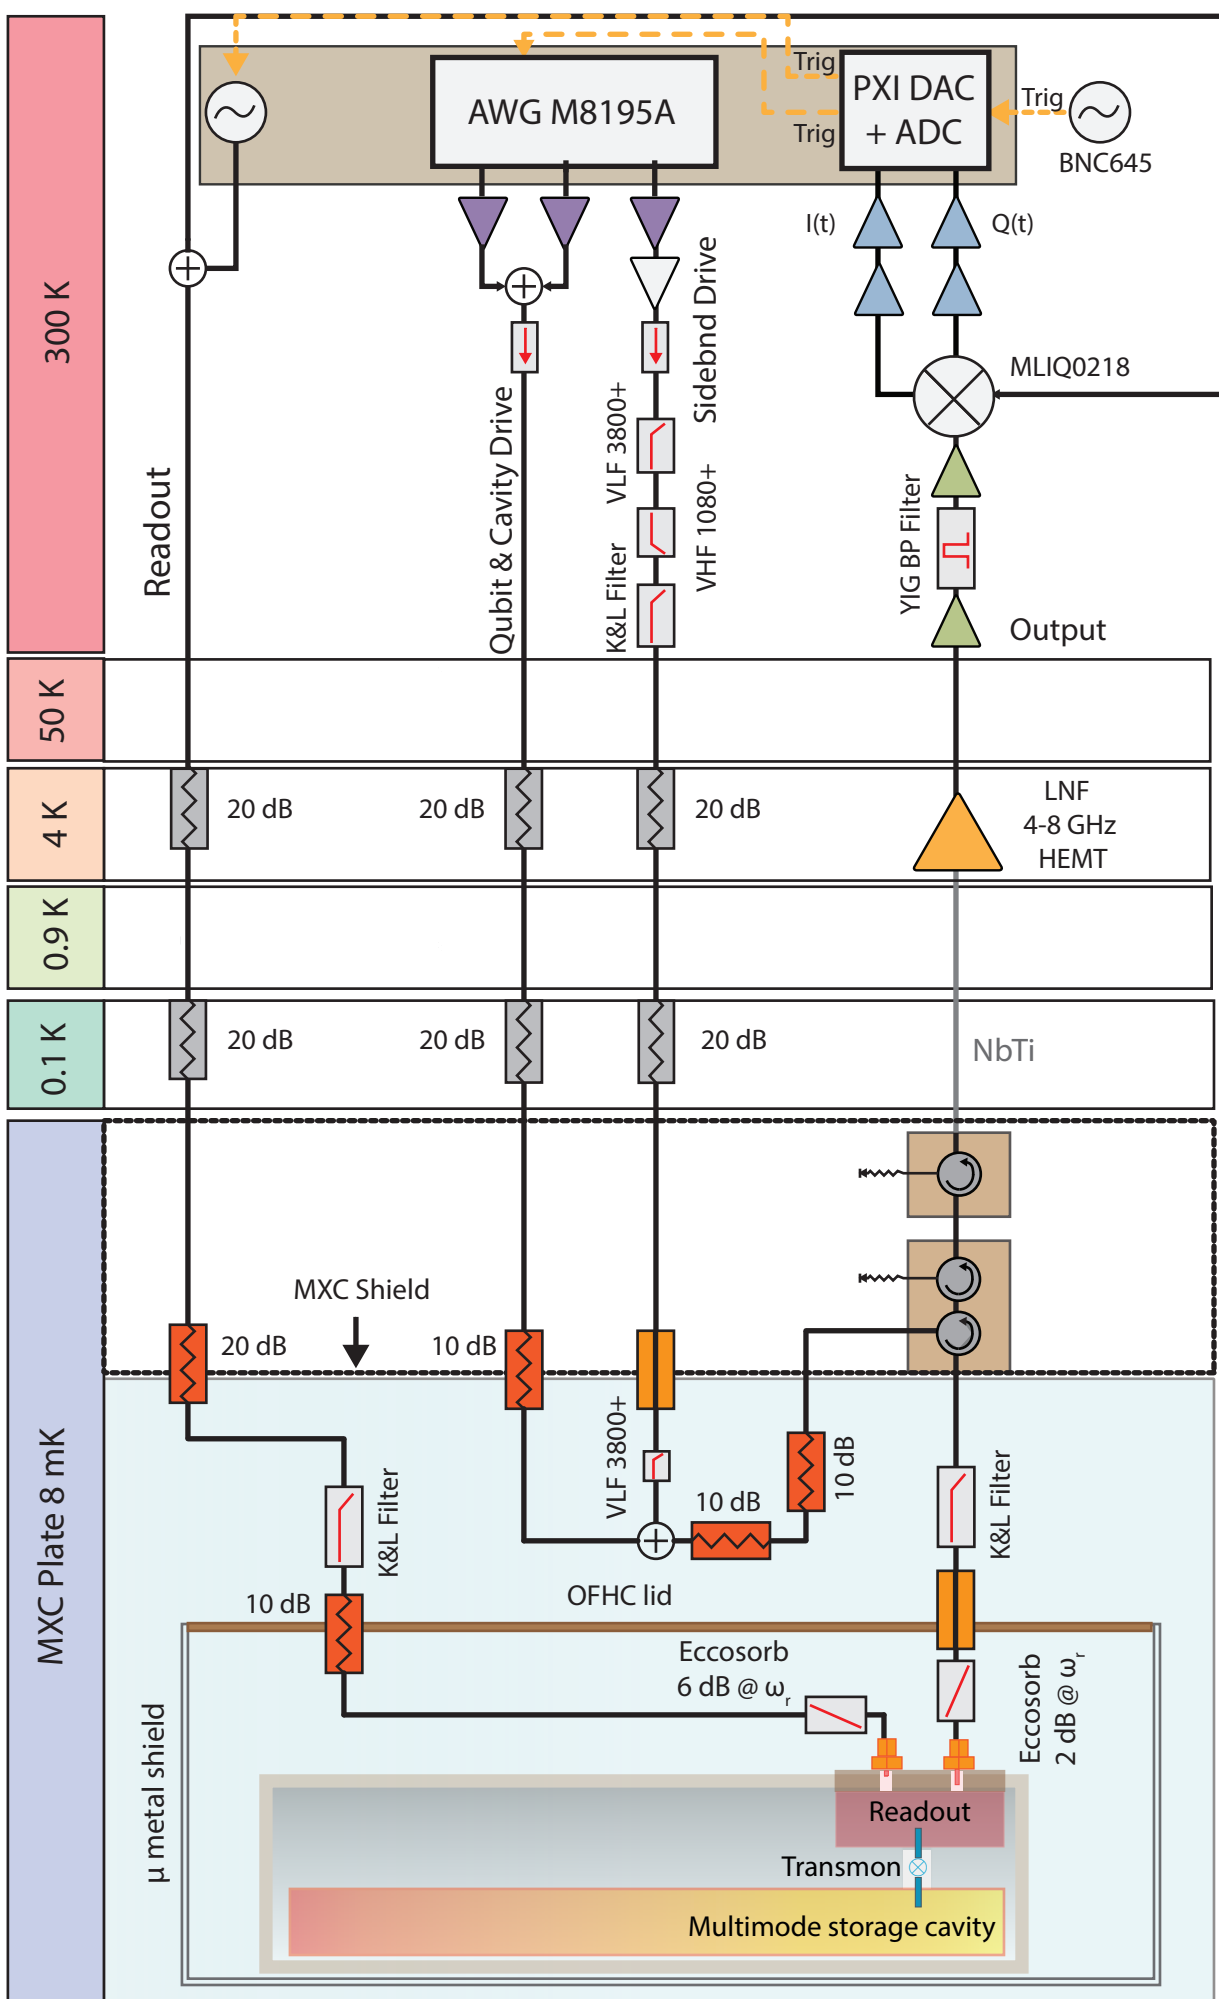

The AWGs, LOs and the trigger are synced to an SRS FS275 Rb Source

- 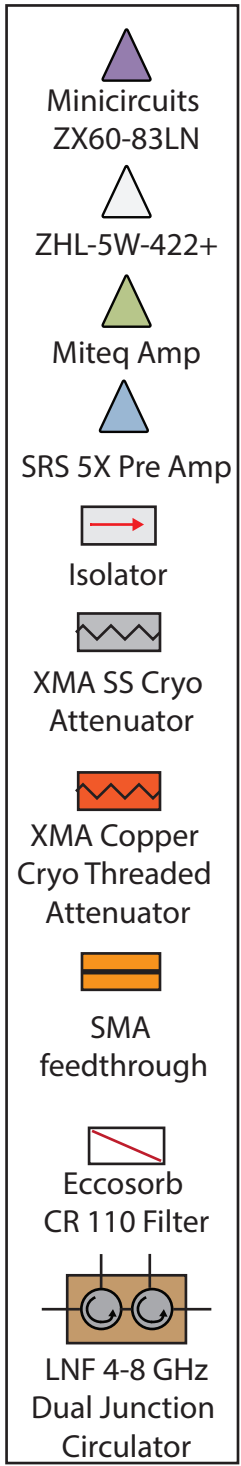 Minicircuits ZX60-83LN
- 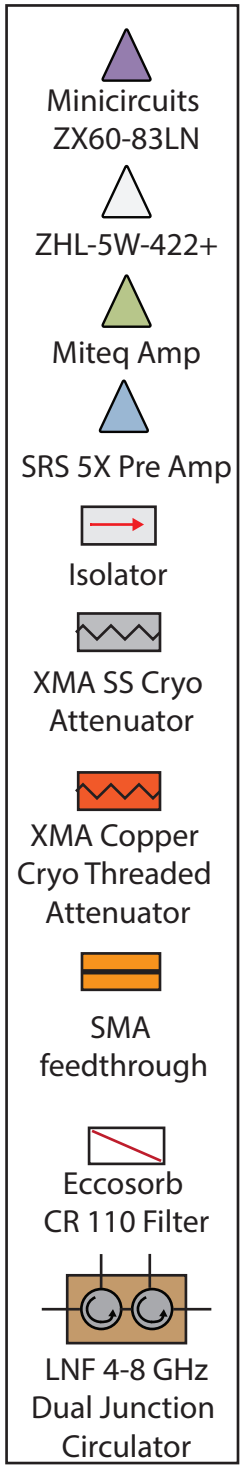 ZHL-5W-422+
- 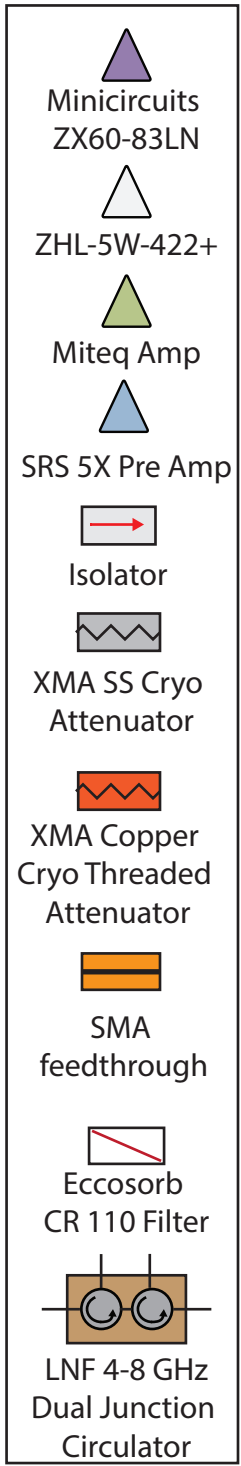 Miteq Amp
- 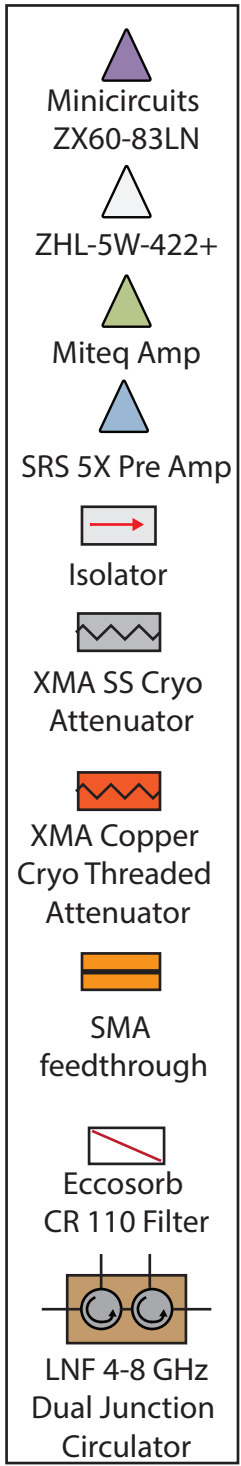 SRS 5X Pre Amp
- 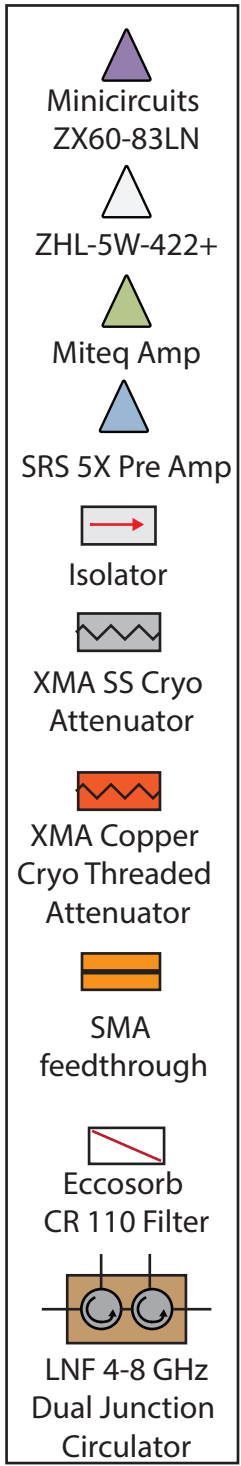 Isolator
- 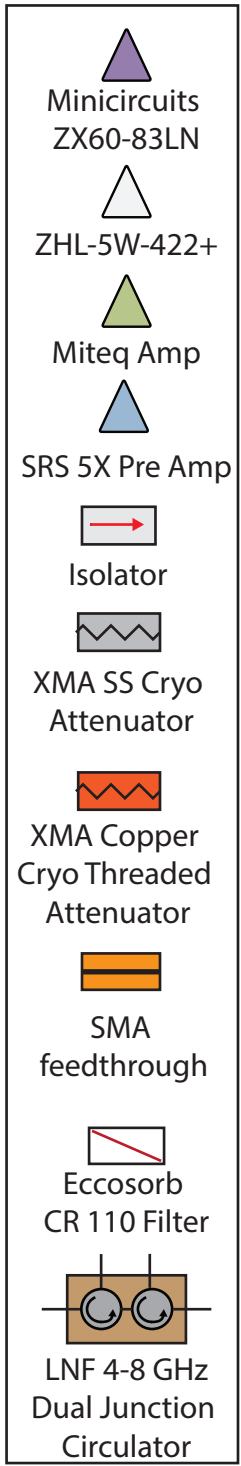 XMA SS Cryo Attenuator
- 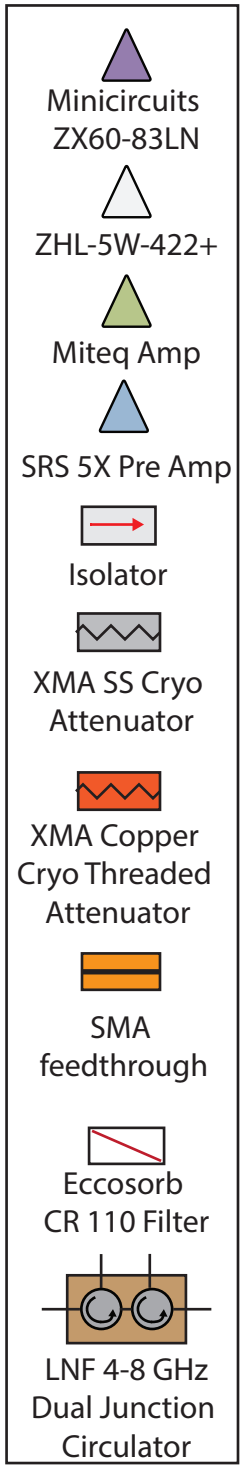 XMA Copper Cryo Threaded Attenuator
- 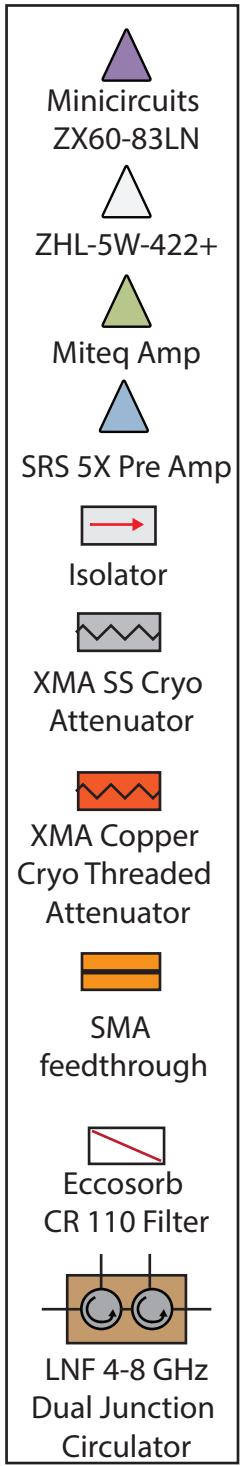 SMA feedthrough
- 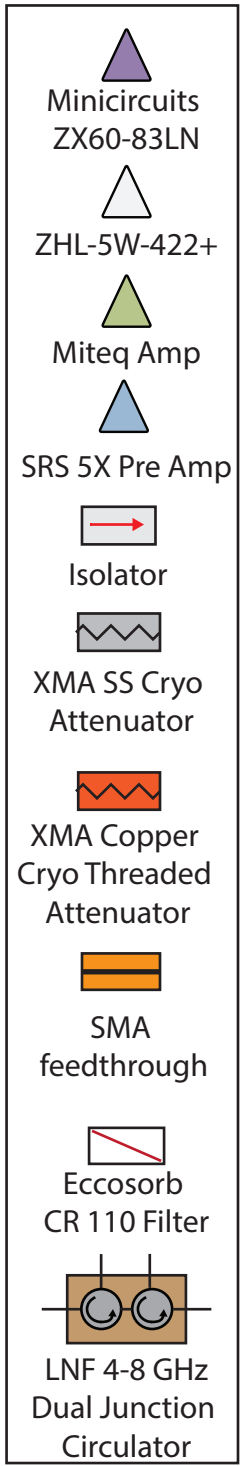 Eccosorb CR 110 Filter
- 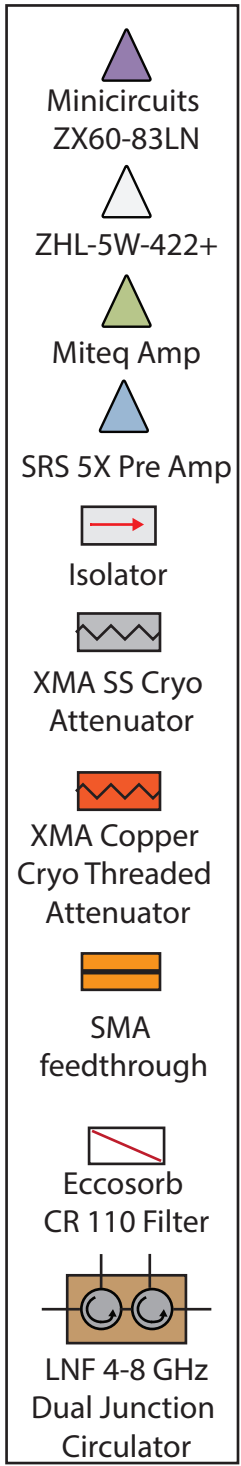 LNF 4-8 GHz Dual Junction Circulator

MXC Plate 800

MXC Plate 800

MXC Plate 800

MXC Plate 800
